# Supplementary material for: Nondeterministic Polynomial-time Problem Challenge: An Ever-Scaling Reasoning Benchmark for LLMs
Source: arXiv:2504.11239 source file (2026-02-08)
Supplement: Supplementary file 1 [file cost.tex]

\begin{table}[ht]
\centering
\caption{Cost for online models}
\label{tab:cost_online}
\begin{tabular}{c|c|c|c}
\toprule
Model & Prompt & Completion & Cost \\
\midrule
GPT-4o-mini&30964144 (\$0.15/MTok) & 9442548 (\$0.6/MTok) & \$10.31 \\
GPT-4o&30963606 (\$2.5/MTok) & 7786156 (\$10/MTok) & \$155.27 \\
Claude-3.7-Sonnet&33799101 (\$3/MTok) & 11186272 (\$15/MTok) & \$269.19 \\
DeepSeek-V3&31490957 (2RMB/MTok)& 16178388 (8RMB/MTok)& 192.41RMB \\
DeepSeek-V3-2503&31490957 (2RMB/MTok)& 31808451 (8RMB/MTok)& 317.45RMB \\
DeepSeek-R1&31512557 (4RMB/MTok)& 95936418 (16RMB/MTok)& 1661.03RMB \\
o1-mini&31360984 (\$1.1/MTok) & 35161551 (\$4.4/MTok) & \$189.21 \\
o3-mini&31199884 (\$1.1/MTok) & 110944621 (\$4.4/MTok) & \$522.48 \\

\bottomrule
\end{tabular}
\end{table}
