# Supplementary material for: Nondeterministic Polynomial-time Problem Challenge: An Ever-Scaling Reasoning Benchmark for LLMs
Source: arXiv:2504.11239 source file (2026-02-08)
Supplement: Supplementary file 2 [file leaderboard.tex]

We only provide the screenshot of the leaderboard in Figure~\ref{fig:leaderboard} due to the anonymity of the submission. We will release this leaderboard upon the acceptance of the paper. 

\begin{figure}[ht]
    \centering
    \includegraphics[width=\linewidth]{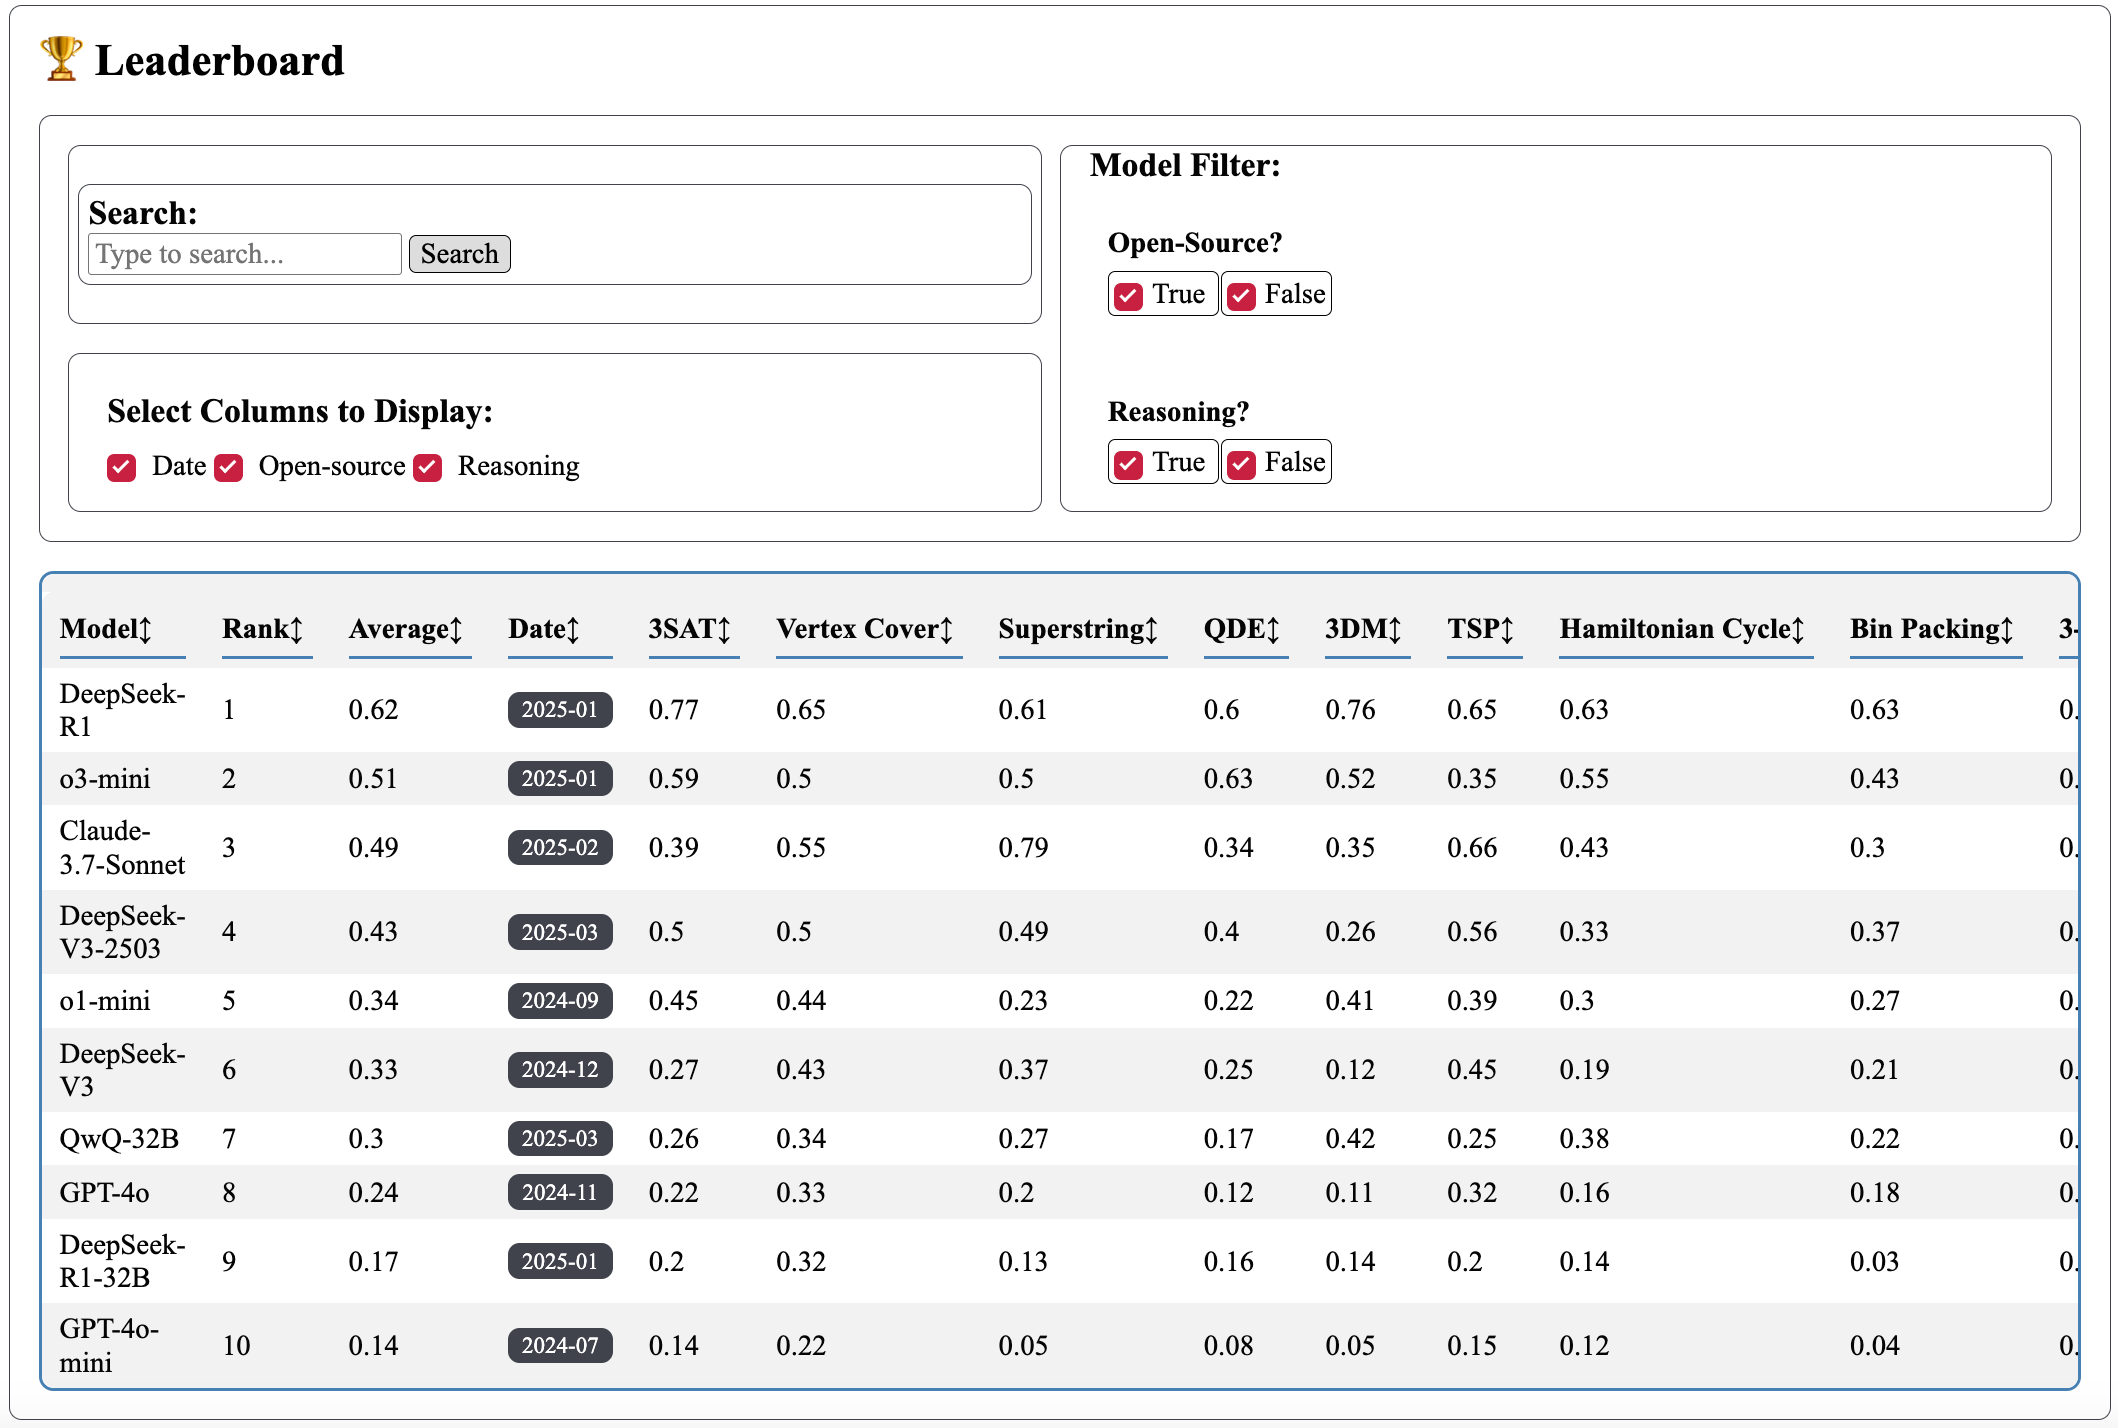}
    \caption{Screenshot of \textbf{NPPC} leaderboard}
    \label{fig:leaderboard}
\end{figure}
